# Supplementary material for: Boosting Object Detection with Zero-Shot Day-Night Domain Adaptation
Source: arXiv:2312.01220 source file (2024-03-27)
Supplement: Supplementary file 1 [file suppdecomnet.tex]

\begin{table}[t]

\begin{minipage}{0.49\linewidth}
    
\centering
    % \scriptsize
    % \setlength{\tabcolsep}{2.5mm}
    % \vspace{-5px}
    % \resizebox{\linewidth}{!}{

	\begin{tabular}{c|c}
    
		\toprule
		Method & mAP(\%)\\
	\midrule
        Ours & 23.5\\
        w/ RF & 24.2\\
    \bottomrule
	\end{tabular}
    % }
    % \vspace{-10px}

    	\caption{Alternative of Retinex decomposition net.}

\label{tab:ablationdecomnet}

\end{minipage}
\hfill
\begin{minipage}{0.49\linewidth}
    
\centering
    % \scriptsize
    % \setlength{\tabcolsep}{2.5mm}
    % \vspace{-5px}
    % \resizebox{\linewidth}{!}{

	\begin{tabular}{c|c}
    
		\toprule
		Method & mAP(\%)\\
	\midrule
        HLA-Face & 44.4\\
        Ours & 44.8\\
    \bottomrule
	\end{tabular}
    % }
    % \vspace{-10px}

    	\caption{Comparison in unsupervised domain adaptation.}
  
\label{tab:compda}

\end{minipage}

\end{table}
